# Supplementary material for: Kinetic freeze-out of the $\phi(1020)$ meson in Pb-Pb collisions at $\sqrt{s_{\rm NN}} = 2.76$ TeV: a blast-wave and hybrid-model study
Source: arXiv:2606.31175 source file (2026-11-13)
Supplement: Supplementary file 1 [file supplemental.tex]

% ****** Supplemental Material for PRL Letter ******
\documentclass[aps,prl,twocolumn,superscriptaddress]{revtex4-2}

\usepackage{graphicx}
\usepackage{amsmath}
\usepackage{amssymb}
\usepackage{hyperref}
\usepackage{xcolor}
\usepackage{multirow}

% Math macros (same as main)
\newcommand{\sqrts}{\sqrt{s_{\rm NN}}}
\newcommand{\Tkin}{T_{\rm kin}}
\newcommand{\Tch}{T_{\rm ch}}
\newcommand{\dT}{\Delta T}

\newcommand{\bs}{\beta_s}
\newcommand{\betaavg}[1][]{\langle\beta\ifx\\#1\\\else_{#1}\fi\rangle}
\newcommand{\betaavgbulk}{\langle\beta^{\rm bulk}\rangle}
\newcommand{\pT}{p_{\rm T}}
\newcommand{\mT}{m_{\rm T}}
\newcommand{\Tstrut}{\rule{0pt}{2.6ex}}
\newcommand{\Bstrut}{\rule[-1.2ex]{0pt}{0pt}}

\begin{document}

\title{Supplemental Material:\\
Evidence for differential kinetic freeze-out
of the \texorpdfstring{$\phi(1020)$}{phi(1020)} meson in
Pb--Pb collisions at \texorpdfstring{$\sqrts = 2.76$}{sqrt(s_NN) = 2.76}~TeV}

\author{Neeraj}
\author{Amal Sarkar}
\affiliation{Indian Institute of Technology Mandi, Kamand,
Himachal Pradesh, India}

\maketitle

This Supplemental Material provides additional details on the analysis methodology, systematic checks, and extended results that support the main Letter.

% ═══════════════════════════════════════════════════════════
\section{BGBW Formalism and Fitting Procedure}
\label{sec:formalism}

The Boltzmann--Gibbs blast-wave (BGBW) model describes a thermalized fireball with collective radial flow at kinetic freeze-out~\cite{Schnedermann:1993ws,Florkowski:2006}. The invariant yield as a function of $\pT$ is
\begin{align}
\frac{d^2 N}{2\pi\,\pT\,d\pT\,dy} &=
\frac{A}{(2\pi)^2}\int_0^R r\,dr\,\mT \notag\\
&\times I_0\!\left(\frac{\pT\sinh\rho}{T}\right)
K_1\!\left(\frac{\mT\cosh\rho}{T}\right),
\end{align}
where $\mT = \sqrt{\pT^2 + m^2}$ is the transverse mass, $I_0$ and $K_1$ are modified Bessel functions, $r/R \in [0,1]$ is the normalized radial position, and $\rho = \tanh^{-1}[\bs \, (r/R)^n]$ is the dimensionless boost rapidity at radius $r$, $\bs$ is the surface velocity, $n$ is the flow profile exponent, $T$ is the kinetic freeze-out temperature, and $A$ is a normalization constant. The average transverse velocity is $\betaavg = \frac{2}{2+n}\bs$. The integration is performed numerically using 16-point Gauss--Legendre quadrature.

\subsection{Fitting procedure}

We perform a $\chi^2$ grid scan on a $200 \times 200$ mesh in $(T, \betaavg)$ with $T \in [60, 230]$~MeV and $\betaavg \in [0.30, 0.80]$, at fixed $n = n^{\rm bulk}$. At each point on the grid, the normalization $A$ is determined analytically: $A = \sum_i y_i f_i/\sigma_i^2 \big/ \sum_i f_i^2/\sigma_i^2$,
and
\begin{equation}
\chi^2 = \sum_{i=1}^{N_{\rm pts}}
\left(\frac{y_i - A\,f_i(\pT^i; T, \bs, n)}{\sigma_i}\right)^2,
\end{equation}
where $y_i \pm \sigma_i$ are the experimental data points (statistical and systematic uncertainties added in quadrature) and $f_i$ is the prediction of the BGBW model.

\subsection{Bootstrap confidence intervals}

The confidence intervals in $(T, \betaavg)$ are obtained by bootstrap resampling~\cite{Efron:1993}. For each of the bootstrap replicas $N_{\rm boot} = 2000$, the replacement data points $N$, and the grid scan are repeated to find the best-fit parameters. The 95\% confidence interval is defined by the 2.5\% and 97.5\% quantiles of the bootstrap distribution.

% ═══════════════════════════════════════════════════════════
\section{Data Sources}

\subsection{Bulk parameters}

The reference bulk freeze-out parameters ($\Tkin, \betaavg, n$) are obtained from a simultaneous BGBW fit to published ALICE $\pi/K/p$ spectra at 0--5\% centrality~\cite{ALICE:2013mez}: $\Tkin = 93.6 \pm 4.9$~MeV, $\betaavg = 0.651 \pm 0.014$, $n = 0.71 \pm 0.05$, $\chi^2/\text{ndf} = 1.14$.

\subsection{\texorpdfstring{$\phi(1020)$}{phi(1020)} spectrum}

The $\pT$ spectrum of $\phi(1020)$ in 0--5\% centrality Pb--Pb at $\sqrts = 2.76$~TeV is from Ref.~\cite{ALICE:2014jbq_phi}, using six data points in the range $0.8 < \pT < 3.5$~GeV/$c$. This centrality bin is identical to the bulk fit, ensuring that there is no centrality-mismatch systematic.

\subsection{Other strange species}

The $\Lambda$, $\Xi$, and $\Omega$ spectra are from Ref.~\cite{ALICE:2014jbq}. None produces a model-adequate BGBW fit at this energy. The failure mode is different for each species and reflects its position in the rescattering hierarchy.

\textit{$\Lambda$.}---With $\chi^2/\text{ndf} > 500$, the $\Lambda$ spectrum is catastrophically inconsistent with
BGBW at this energy. $\Lambda$ has a large feed-down contribution from $\Sigma^0 \to \Lambda\gamma$ and weak-decay feed-in from hyperon cascades; these non-thermal sources distort the low-$\pT$ shape and make a thermal fit meaningless.

\textit{$\Xi$.}---The $\Xi$ fit gives $\chi^2/\text{ndf} = 19.3$ (6 data points, 2 free parameters), indicating a severe spectral mismatch. With hadronic cross section $\sigma_{\Xi} \approx 12$~mb and estimated rescattering depth $N_{\rm scatt} \sim 3$ (using $n_{\rm hadron} = 0.34$~fm$^{-3}$, $L_{\rm eff} = \frac{4}{3}R_{\rm side}$,
$R_{\rm side} = 6.2$~fm), $\Xi$ undergoes enough interactions to populate the high-$\pT$ tail through successive momentum transfers. The $\pT$-range systematics shown in Fig.~\ref{fig:pt_sys} confirm this diagnosis: $\Tkin^{\Xi}$ is highly sensitive to the upper $\pT$ cut, increasing from $\sim\!14$~MeV at $\pT^{\rm hi} = 3.5$~GeV/$c$ to $\sim\!62$~MeV at $\pT^{\rm hi} = 3.0$~GeV/$c$. This identifies jet fragmentation and coalescence contributions at $\pT \gtrsim 3$~GeV/$c$ as the source of model failure. Replacing BGBW with the Tsallis blast-wave also gives $\chi^2/\text{ndf} \geq 55$ for $\Xi$, confirming that the failure is not model-specific but reflects genuine non-thermal features of the spectrum.

\textit{$\Omega$.}---Only 8 data points are available in the range $1.3 \leq \pT \leq 3.4$~GeV/$c$ (application of the same upper cut of $3.5$~GeV/$c$ used for $\phi$ and $\Xi$), making the 2-parameter BGBW fit marginally constrained with 6~degrees of freedom. The nominal $\chi^2/\text{ndf} = 0.8$ is therefore not a meaningful measure of adequacy of the model. With $\sigma_{\Omega} \approx 5$~mb and $N_{\rm scatt} \sim 1.4$, $\Omega$ is too transparent to reliably thermalize; therefore, no exclusion statement similar to $\phi$ can be made. These failure modes are summarized alongside the rescattering estimates in Table~2 of the main Letter.

% ═══════════════════════════════════════════════════════════
\section{Robustness Checks}
\label{sec:robustness}

\subsection{\texorpdfstring{$\pT$}{pT} range variation}

To assess the sensitivity of $\dT$ to the choice of fit range, we vary the low-$\pT$ cut ($0.5$--$1.0$~GeV/$c$) and
high-$\pT$ cut ($2.5$--$4.5$~GeV/$c$) independently, using $\Xi$ as diagnostic control alongside $\phi$.

Figure~\ref{fig:pt_sys} reveals a sharp asymmetry: $\Tkin^{\Xi}$ increases substantially when the upper cut is reduced below 3.5~GeV/$c$, while varying the lower cut by 0.4~GeV/$c$ changes $\Tkin^{\Xi}$ by only $\sim5$~MeV.
This identifies the high-$\pT$ tail ($\pT \gtrsim 3$~GeV/$c$) as the source of model failure for $\Xi$: non-thermal contributions from jet fragmentation and coalescence pull the fitted temperature downward, producing the misleadingly low nominal $\Tkin^{\Xi}$.

By contrast, $\Tkin^{\phi}$ varies only by $\sim 26$~MeV throughout the whole grid, remaining well above $\Tkin^{\rm bulk}$ at every range combination. The $K\bar{K}$ reconstruction requirement suppresses hard-scattering backgrounds throughout the fitted $\pT$ range, making $\phi$ spectrally clean and its fitted temperature robust against range choice.

\begin{figure}[htbp]
\centering
\includegraphics[width=\columnwidth]{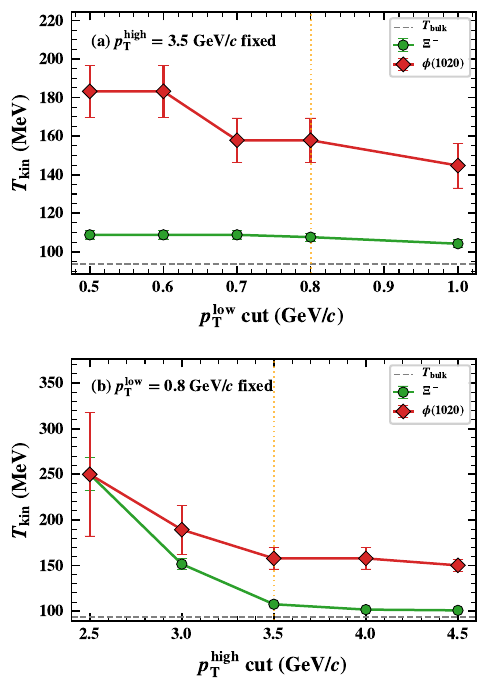}
\caption{Fitted kinetic freeze-out temperature $\Tkin$ as a
function of the $\pT$ fit range, for $\phi(1020)$ (red diamonds)
and $\Xi^-$ (green circles) in 0--5\% Pb--Pb at
$\sqrts = 2.76$~TeV.
Panel~(a): $\Tkin$ vs.\ the low-$\pT$ cut
  (high-$\pT$ fixed at 3.5~GeV/$c$).
Panel~(b): $\Tkin$ vs.\ the high-$\pT$ cut
  (low-$\pT$ fixed at 0.8~GeV/$c$).
The dashed line marks $\Tkin^{\rm bulk} = 93.6$~MeV.
The orange dotted line indicates the nominal cut.
$\phi$ is insensitive to range choice; $\Xi$ exhibits
a strong dependence on the high-$\pT$ cut,
indicating contamination from non-thermal tails.
\label{fig:pt_sys}}
\end{figure}

\subsection{Flow profile exponent (\texorpdfstring{$n$}{n}-scan)}

Scanning $n \in [0.20, 0.90]$ (the entire physically meaningful range), we find $\Delta\chi^2 \geq 6.2$ at all values (Table~\ref{tab:nscan}). At $n = 0.50$, the displacement is $\Delta\chi^2 = 141$; at $n = n^{\rm bulk} = 0.71$, it is 21.7. For $n \leq n^{\rm bulk}$, the displacement manifests as $\betaavg[\phi] > \betaavgbulk$ (harder spectrum through increased flow; $\Delta\chi^2 > 100$); for $n > n^{\rm bulk}$, the minimum shifts to higher $T$ (harder spectrum through higher temperature), reflecting the rotation of the $T$--$\bs$ degeneracy ridge. At $n = 0.90$, the compression of the ridge reduces $\Delta\chi^2$ to 6.2, marginally above the 95\% CL threshold. The exclusion is robust to the choice of flow profile across the full scan range.

\begin{table}[htbp]
\caption{$\Delta\chi^2$ at the bulk $(T, \betaavg)$ point for the $\phi(1020)$ fit at each fixed $n$ (same methodology as the main contour figure). All values exceed the 95\% CL threshold of 6.0. Entries with $\Tkin > \Tch \approx 156$~MeV are marked ($\dagger$) and excluded from the primary
robustness claim.
\label{tab:nscan}}
\begin{ruledtabular}
\begin{tabular}{ccccc}
$n$ & $\Tkin^\phi$ (MeV) & $\betaavg[\phi]$ &
$\chi^2_{\rm min}$ & $\Delta\chi^2$ \Tstrut \Bstrut\\
\hline
0.20 & 175.4$^\dagger$ & 0.729 & 0.3 & 206 \\
0.30 & 156.2$^\dagger$ & 0.729 & 0.2 & 191 \\
0.40 & 130.3 & 0.729 & 0.2 & 170 \\
0.50 &  98.7 & 0.725 & 0.4 & 141 \\
0.60 &  82.6 & 0.710 & 1.6 & 102 \\
0.71 &  89.4 & 0.681 & 5.0 &  43 \\
0.80 & 102.7 & 0.659 & 7.7 & 9.2 \\
0.90 & 127.1 & 0.632 & 11.3 & 6.2 \Bstrut\\
\end{tabular}
\end{ruledtabular}
\end{table}

\subsection{\texorpdfstring{$K\bar{K}$}{KKbar} regeneration}

If 15\% of the $\phi$ yield originates from
post-freeze-out $K\bar{K}$ coalescence,
reducing the effective $\phi$ yield at low $\pT$,
the displacement decreases to
$\Delta\chi^2 \sim 17$, still well above the
two-parameter 95\% CL threshold of $\Delta\chi^2 = 6.0$.
The exclusion of the bulk freeze-out point therefore
remains significant even under this conservative scenario.

\subsection{Bulk point variation}

Shifting the bulk point within its statistical uncertainties ($\pm 5$~MeV in $T$, $\pm 0.015$ in $\betaavg$) changes $\Delta\chi^2$ from 21.7 to 15--28, well above the 95\% threshold.

% ═══════════════════════════════════════════════════════════
\section{Tsallis Blast-Wave Check}

To verify model independence, the BGBW has been replaced with the Tsallis blast-wave (TBW) parameterization, which substitutes the Boltzmann factor $e^{-E/T}$ with the Tsallis distribution $(1 + (q-1)E/T)^{-1/(q-1)}$~\cite{Tang:2009TBW}. Scanning $q \in [1.00, 1.10]$ with $(T, \text{norm})$ free at each $q$ (fixing $\bs$, and $n$ at bulk values), we find $\Delta\chi^2 \geq 23$ at the bulk point throughout the scan (Table~\ref{tab:tbw}), with $\Delta\chi^2 = 47$ at the optimal $q = 1.015$. These values exceed the 2-parameter 95\% CL threshold of 6.0 by factors of 4--29, confirming that the $\phi$--bulk displacement is not an artifact of the BGBW model choice.

\begin{table}[htbp]
\caption{TBW model independence check: $\Delta\chi^2$ at the bulk $(T, \betaavg)$ point for $\phi(1020)$
at different values of the non-extensivity parameter $q$.
All values exceed the 95\% CL threshold of 6.0.
\label{tab:tbw}}
\begin{ruledtabular}
\begin{tabular}{ccccc}
$q$ & $\Tkin^\phi$ (MeV) & $\betaavg[\phi]$ &
$\chi^2_{\rm min}$ & $\Delta\chi^2$ \Tstrut \Bstrut \\
\hline
1.000 & 171.9 & 0.566 & 0.24 &  23 \\
1.015 & 145.1 & 0.573 & 0.24 &  47 \\
1.020 & 137.2 & 0.575 & 0.24 &  57 \\
1.040 & 103.1 & 0.583 & 0.27 &  96 \\
1.060 &  72.1 & 0.589 & 0.32 & 130 \\
1.080 &  60.0 & 0.573 & 0.87 & 158 \\
1.100 &  60.0 & 0.540 & 3.42 & 177 \Bstrut \\
\end{tabular}
\end{ruledtabular}
\end{table}

The $\Xi$ baryon also remains poorly described ($\chi^2/\text{ndf} \geq 55$) under TBW, confirming that its model inadequacy is not specific to the BGBW functional form, but reflects genuine spectral features (feed-down, non-thermal tails) that no blast-wave variant can accommodate.

% ═══════════════════════════════════════════════════════════
\section{\texorpdfstring{$T$--$\beta$}{T-beta} Degeneracy and Rescattering Depth}

The BGBW model exhibits an intrinsic $T$--$\betaavg$ anti-correlation: increasing temperature can be compensated by reducing the flow to produce similar spectral shapes. For $\phi$, this degeneracy manifests as a $\chi^2$ ridge spanning $(T, \betaavg) \approx (60\text{--}150\;\text{MeV},\; 0.65\text{--}0.69)$, passing through both the free-$\bs$ minimum $(\approx 90, 0.68)$ and the fixed-$\bs$ solution $(150, 0.65)$. Neither endpoint uniquely determines the physical freeze-out mechanism; only the \textit{displacement} of the entire ridge from the bulk point is model-independent.

The direction of the ridge can be understood physically: a particle with $n_{\rm scatt}$ rescatterings after chemical freeze-out acquires collective flow that scales with the number of interactions, while its effective temperature decreases as the fireball cools~\cite{Heinz:2008}. The $\phi$, with $\sigma_{\phi\text{-hadron}} \lesssim 2$~mb~\cite{STAR:2026BES2} versus $\sigma_{\pi N} \sim 30$~mb for pions, undergoes fewer rescatterings than $\pi$ or $K$, naturally resulting in either a higher $T$ or weaker flow, exactly along the observed ridge direction.

We estimate the number of hadronic rescatterings as 
\begin{equation}
N_{\rm scatt} = \sigma \cdot n_{\rm hadron} \cdot L_{\rm eff},
\end{equation}
where $n_{\rm hadron} \approx 0.34$~fm$^{-3}$ is the density of the hadron at chemical freeze-out~\cite{Andronic:2018} and $L_{\rm eff} = \frac{4}{3}R_{\rm side}$ is the mean chord length through the freeze-out volume~\cite{deKruijf:2003}, with $R_{\rm side} = 6.2 \pm 0.5$~fm from the ALICE HBT measurements~\cite{ALICE:2011HBT}. This yields $N_{\rm scatt} \sim 0.5$ for $\phi$, $\sim 1.4$ for $\Omega$, $\sim 3$ for $\Xi$, and $\sim 4$--$11$ for bulk hadrons---consistent with the observed pattern of BGBW fit quality: $\phi$ undergoes just enough rescattering to partially thermalize while remaining decoupled from the bulk cooling, while $\Omega$ is too transparent to fully thermalize. These estimates are upper bounds because the straight-line chord approximation overestimates the actual path through the dense hadronic phase.

% ═══════════════════════════════════════════════════════════
\section{Systematic Uncertainties Summary}
Since the primary result is the displacement of $\phi$ from the bulk in the $(T, \betaavg)$ space, $T$--$\beta$ is not treated as a systematic uncertainty; it is resolved by the full 2D contour analysis. The remaining systematic uncertainties on the $\phi$ contour position are summarized in Table~\ref{tab:sys}.

\begin{table}[htbp]
\caption{Systematic uncertainties affecting the $\phi$
contour position at 0--5\% centrality.\label{tab:sys}}
\begin{ruledtabular}
\begin{tabular}{p{3.6cm}c}
Source & Impact \Tstrut \Bstrut\\
\hline
$\pT$ range variation
  & $\Tkin^\phi$: 64--90~MeV \\
$K\bar{K}$ regen.\ (15\%)
  & $\Delta\chi^2$: $21.7 \to {\sim}17$ \\
Bootstrap (stat.)
  & $\pm 14$~MeV in $T$ \\
Bulk $(T, \betaavg)$ shift$^{\rm a}$
  & $\Delta\chi^2$: 15--28 \\
Flow profile $n$ scan
  & $\Delta\chi^2 \geq 6.2$ \\
Tsallis BW check
  & $\Delta\chi^2 \geq 23$ \Bstrut\\
\end{tabular}
\end{ruledtabular}
$^{\rm a}${$\pm 5$~MeV in $T$,
$\pm 0.015$ in $\betaavg$.}
\end{table}

% ═══════════════════════════════════════════════════════════
\section{SMASH Simulation Details}

The SMASH~3.3~\cite{Weil:2016SMASH} simulation uses a thermal box ($L = 20$~fm) initialized at $T_{\rm ch} = 156$~MeV~\cite{Andronic:2018}, with hadron multiplicities approximating 0--5\% Pb--Pb at $\sqrts = 2.76$~TeV. The system evolves for 100~fm/$c$; 4500 events (9 runs with independent random seeds) were generated on CERN lxplus. The $\phi$ meson ($\tau_\phi \approx 46$~fm/$c$) decays before the output time; its spectrum is reconstructed from $K^+K^-$ invariant-mass pairs with
$|m_{K^+K^-} - m_\phi| < 6$~MeV ($\approx 1.4\,\Gamma_\phi$) and geometric-mean like-sign background subtraction ($N_{\rm signal} = N_{+-} - 2\sqrt{N_{++}N_{--}}$)~\cite{ALICE:2015PhiKstar}. The effective temperature is extracted from a Boltzmann fit: $dN/(2\pi\,\pT\,d\pT\,dy) \propto \mT\,K_1(\mT/T_{\rm eff})$.
\bibliography{apssamp}

\end{document}
